# Supplementary material for: Neural Model-based Optimization with Right-Censored Observations
Source: arXiv:2009.13828 source file (2020-09-29)
Supplement: Supplementary file 1 [file appendix.pdf]

# Appendix: Neural Model-based Optimization with Right-Censored Observations

**Katharina Eggensperger,[1] Kai Haase,[1] Philipp Müller,[1] Marius Lindauer,[2] Frank Hutter[1,3]**
[1] University of Freiburg, Germany
[2] Leibniz University Hannover, Germany
[3] Bosch Center for Artificial Intelligence
eggenspk@cs.uni-freiburg.de, haasek@informatik.uni-freiburg.de, muelleph@informatik.uni-freiburg.de,
lindauer@tnt.uni-hannover.de, fh@cs.uni-freiburg.de

## More details for *Studying the Impact of Censored Observations*

Here, we provide additional results for evaluating the predictive quality of our NNs on actual data obtained during optimization. Based on the same experiments as in the main paper, we plot the L2 loss between the predicted median and the empirical median (as a more robust metric when observing censored data) and the RMSE when only considering configurations for which the mean performance is better than the global cutoff value (to provide an alternative measurement that takes only the actually observed performance range into account).

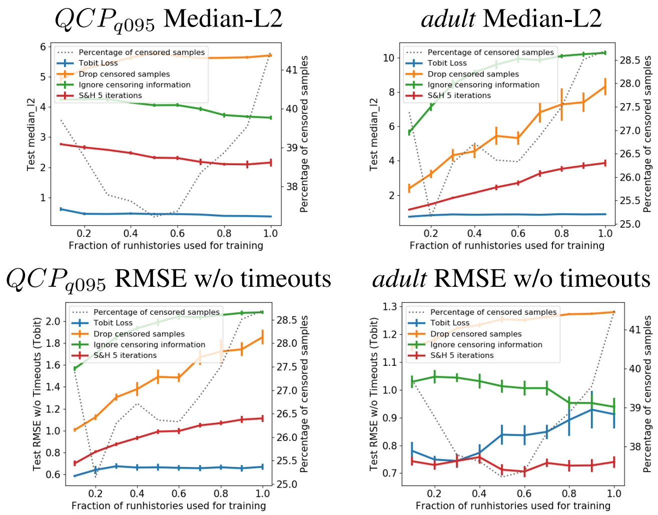


Figure 1: Results for I, D, S&H and T on actual runtime data. The upper plots show L2 loss w.r.t. the empirical and predicted median and the lower plots show RMSE w/o timeouts when training on increasing fractions of observed data during optimization and tested on unseen data from the same distribution.

## More details for *Model-based Optimization*

Here, we provide the configuration spaces used for tuning the number of steps for *Saps* (Table 2) and for tuning time-to-accuracy for neural networks (Table 1). Furthermore, analogously to Table 2 in the main paper, we provide in Table 3 for each optimization problems the median score, which describes the percentage of the best found configuration per run and the overall best found function value normalized between the best and worst found configuration per scenario.

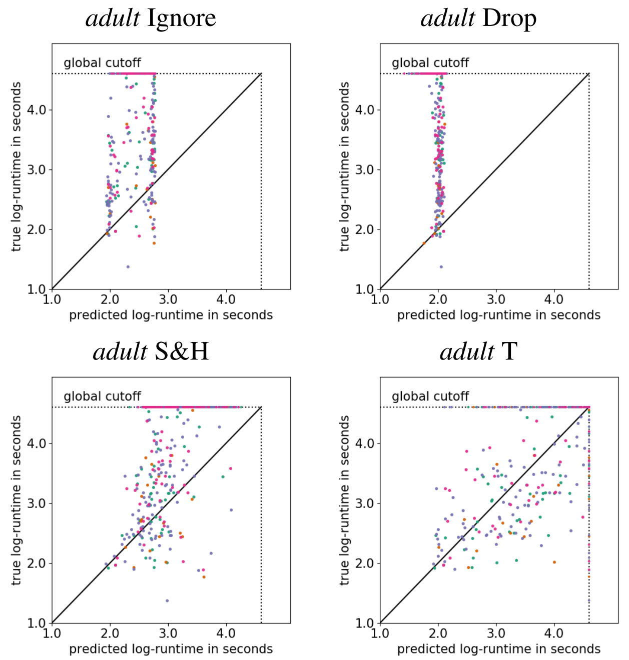


Figure 2: Results for I, D, S&H and T. We show predicted values versus true observations on a log-scale for training on 100% of the data obtained on the time-to-acurracy benchmark *adult*.

Table 1: 4-dimensional searchspace for tuning *Saps*.

| **name** | **range** | **default** | **type** | **log** |
|---|---|---|---|---|
| alpha | $[1, 1.4]$ | 1.3 | float | ✓ |
| rho | $[0, 1]$ | 0.8 | float | ✗ |
| ps | $[0, 0.2]$ | 0.05 | float | ✗ |
| wp | $[0, 0.06]$ | 0.01 | float | ✗ |

Table 2: 7-dimensional searchspace for tuning neural networks.

| **name** | **range** | **default** | **type** | **log** |
|---|---|---|---|---|
| batch size | $[16, 512]$ | 32 | int | ✓ |
| learning rate | $[1e^{-4}, 1e^{-1}]$ | $1e^{-3}$ | float | ✓ |
| momentum | $[0.1, 0.99]$ | 0.99 | float | ✗ |
| weight decay | $[1e^{-5}, 1e^{-1}]$ | $1e^{-3}$ | float | ✗ |
| #layers | $[1, 5]$ | 2 | int | ✗ |
| #units | $[64, 1024]$ | 128 | int | ✓ |
| dropout | $[0.0, 1.0]$ | 0.5 | float | ✗ |

Table 3: Results for minimizing number of steps for *Saps* (upper) and the time-to-accuracy for NNs (lower), see Table 2 in the main paper. We report the averaged score normalized with the best and worse final configuration found by an optimization procedure. For each optimization method we report the median, the lower and upper quartiles across repetitions. For *Saps*, we conducted 32 runs and evaluated the final configuration 1 000 times run with a different seed while for the NNs, we conducted 16 runs and evaluated each configuration 100 times run with a different seed. We underline the best found value and boldface values that are not statistically different due to a random permutation test with 100 000 permutations.

| Set | Rand | RF w\ S&H | NN w\ TS & Tobit |
|---|---|---|---|
| $QCP_{med}$ | 70.21 | 70.65 | **86.74** |
| $QCP_{q075}$ | **94.0** | **95.23** | **97.97** |
| $QCP_{q095}$ | **99.65** | **99.66** | **99.86** |
| adult | 16.37 | 88.22 | **97.91** |
| airlines | 43.07 | **79.59** | **95.91** |
| bank | 30.75 | 69.5 | **83.74** |
| connect-4 | 55.22 | **90.66** | **78.89** |
| credit-g | **82.42** | **97.5** | **96.38** |
| jannis | 53.95 | **85.19** | **85.89** |
| numerai | 89.52 | **93.09** | **91.55** |
| vehicle | **66.34** | **77.62** | **91.43** |
| average rank | 3 | $1.\overline{72}$ | $1.\overline{27}$ |
| average score | 63.77 | 86.08 | 91.39 |
